# Supplementary material for: On the Viability of Stochastic Economic Dispatch for Real-Time Energy Market Clearing
Source: arXiv:2308.06386 source file (2024-10-23)
Supplement: Supplementary file 1 [file formulation_BPM.tex]

\section{Nomenclature}
\label{sec:nomenclature}

\subsection{Indices and Sets}
    \begin{abbrv}
        \item[$i \in \mathcal{N}$] Buses
        \item[$g \in \mathcal{G}$] Generators
        \item[$\mathcal{G}_{i}$] Generators at bus $i$
        \item[$e \in \mathcal{E}$] Branches
        \item[$t \in \mathcal{T}$] Time steps
        \item[$s \in \mathcal{S}$] Scenarios
    \end{abbrv}

\subsection{Variables}

    \begin{abbrv}
        \item[$\p_{i,t,s}$] Net active power injection at bus $i$ at time $t$ in scenario $s$ (MW)
        \item[$\pf_{e, t, s}$] Power flow on branch $e$ at time $t$ in scenario $s$ (MW)
        \item[$\pg_{g, t, s}$] Active power dispatch of generator $g$ at time $t$ in scenario $s$ (MW)
        \item[$\pg^{k}_{g, t, s}$] Active power dispatch for piecewise segment $k$ of generator $g$ at time $t$ in scenario $s$ (MW)
        \item[$\reg_{g, t, s}$] Regulating reserve dispatch of generator $g$ at time  $t$ in scenario $s$ (MW)
        \item[$\spin_{g, t, s}$] Spinning reserve dispatch of generator $g$ at time $t$ in scenario $s$ (MW)
        \item[$\suppOn_{g, t, s}$] Supplemental reserve dispatch of generator $g$ at time $t$ in scenario $s$ (MW)
        \item[$\suppOff_{g, t, s}$] Offline supplemental reserve dispatch of generator $g$ at time $t$ in scenario $s$ (MW)
        \item[$\rcup_{g, t, s}$] Ramping-up capability of generator $g$ at time $t$ in scenario $s$ (MW)
        \item[$\rcdn_{g, t, s}$] Ramping-down capability of generator $g$ at time $t$ in scenario $s$ (MW)
        \item[$\rcstr_{g, t, s}$] Short-term ramping capability of generator $g$ at time $t$ in scenario $s$ (MW)
        \item[$\dpp_{t, s}$] Global power balance surplus at time $t$ in scenario $s$ (MW)
        \item[$\dpm_{t, s}$] Global power balance shortage at time $t$ in scenario $s$ (MW)
        \item[$\dreg_{t, s}$] Regulating reserve shortage at time $t$ in scenario $s$ (MW)
        \item[$\dregspin_{t, s}$] Regulating-plus-spinning reserve shortage at time $t$ in scenario $s$ (MW)
        \item[$\dopres_{t, s}$] Operating reserve shortage at time $t$ in scenario $s$ (MW)
        \item[$\drcup_{t, s}$] Ramping-up capability shortage at time $t$ in scenario $s$ (MW)
        \item[$\drcdn_{t, s}$] Ramping-down capability shortage at time $t$ in scenario $s$ (MW)
        \item[$\drcstr_{t, s}$] Short-term ramping capability shortage at time $t$ in scenario $s$ (MW)
        \item[$\df_{e, t, s}$] Thermal limit violation on branch $e$ at time $t$ in scenario $s$ (MW)
    \end{abbrv}

\subsection{Parameters}

    \begin{abbrv}
        \item[$\dt$]
            Duration of a time period (min)
        \item[$p_s$]
            The probability of scenario $s$
        \item[$\pd_{i,t,s}$]
            Active power demand at bus $i$ at time $t$ in scenario $s$ (MW)
        \item[$\sigma_{e,i}$]
            PTDF coefficient for branch $e$ and bus $i$
        \item[$\pfmin_{e,t}$]
            Lower thermal limit on branch $e$ at time $t$ (MW)
        \item[$\pfmax_{e,t}$]
            Upper thermal limit on branch $e$ at time $t$ (MW)
        \item[$\CF_{g, t}$]
            Commitment flag of generator $g$ at time $t$ (binary)
        \item[$\RF_{g, t}$]
            Regulation flag of generator $g$ at time $t$ (binary)
        \item[$\ITF_{g, t}$]
            Intermittent flag of generator $g$ at time $t$ (binary)
        \item[$\regAvail_{g, t}$]
            Whether generator $g$ can provide regulating reserves at time $t$ (binary)
        \item[$\spinAvail_{g, t}$]
            Whether generator $g$ can provide spinning reserves at time $t$ (binary)
        \item[$\suppOnAvail_{g, t}$]
            Whether generator $g$ can provide online supplemental reserves at time $t$ (binary)
        \item[$\suppOffAvail_{g, t}$]
            Whether generator $g$ can provide offline supplemental reserves at time $t$ (binary)
        \item[$\text{pg}_{g,0}$]
            Initial output of generator $g$ (MW)
        \item[$\pgmin_{g,t,s}$]
            Minimum output of generator $g$ at time $t$ in scenario $s$ (MW)
        \item[$\pgmax_{g,t,s}$]
            Maximum output of generator $g$ at time $t$ in scenario $s$ (MW)
        \item[$\pgstep^{k}_{g, t}$]
            Width of $k^{th}$ bid step for generator $g$ at time $t$ (MW)
        \item[$\rrdn_{g,t}$]
            Ramping-down rate of generator $g$ at time $t$ (MW/min)
        \item[$\rrup_{g,t}$]
            Ramping-up rate of generator $g$ at time $t$ (MW/min)
        \item[$\regmax_{g,t}$]
            Maximum regulating reserve dispatch of generator $g$ at time $t$ (MW)
        \item[$\spinmax_{g,t}$]
            Maximum spinning reserve dispatch of generator $g$ at time $t$ (MW)
        \item[$\suppOnmax_{g,t}$]
            Maximum online supplemental reserve dispatch of generator $g$ at time $t$ (MW)
        \item[$\suppOffmax_{g,t}$]
            Maximum offline supplemental reserve dispatch of generator $g$ at time $t$ (MW)
        \item[$\noload_{g,t}$]
            No-load cost of generator $g$ at time $t$ (\$)
        \item[$C^{k}_{g, t}$]
            Energy dispatch cost at bid step $k$ for generator $g$ at time $t$ (\$/MW)
        \item[$\costRegRes_{g, t}$]
            Regulating reserve cost for generator $g$ at time $t$ (\$/MW)
        \item[$\costSpinRes_{g, t}$]
            Spinning reserve cost for generator $g$ at time $t$ (\$/MW)
        \item[$\costSuppOnRes_{g, t}$]
            Supplemental reserve cost for generator $g$ at time $t$ (\$/MW)
        \item[$\costSuppOffRes_{g, t}$]
            Offline supplemental reserve cost for generator $g$ at time $t$ (\$/MW)
        \item[$\regReq_{t}$]
            Regulating reserve requirement at time $t$ (MW)
        \item[$\regSpinReq_{t}$]
            Regulating-plus-spinning reserve requirement at time $t$ (MW)
        \item[$\opResReq_{t}$]
            Operating reserve requirement at time $t$ (MW)
        \item[$\rcupReq_{t}$]
            Ramping-up capability requirement at time $t$ (MW)
        \item[$\rcdnReq_{t}$]
            Ramping-down capability requirement at time $t$ (MW)
        \item[$\rcstrReq_{t}$]
            Short-term ramping capability requirement at time $t$ (MW)        
        \item[$\penaltyPowerShortage$]
            Global energy shortage penalty price (\$/MW)
        \item[$\penaltyPowerSurplus$]
            Global energy surplus penalty price (\$/MW)
        \item[$\penaltyRegRes$]
            Regulating reserve shortage penalty price (\$/MW)
        \item[$\penaltyRegSpinRes$]
            Regulating plus spinning reserve shortage penalty price (\$/MW)
        \item[$\penaltyOpRes$]
            Operating reserve shortage penalty price (\$/MW)
        \item[$\penaltyRCUp$]
            Ramping-up capability shortage penalty price (\$/MW)
        \item[$\penaltyRCDn$]
            Ramping-down capability shortage penalty price (\$/MW)
        \item[$\penaltyRCStr$]
            Short-term ramping capability shortage penalty price (\$/MW)
        \item[$\penaltyFlow_{e,t}$]
            Transmission violation penalty price for branch $e$ at time $t$ (\$/MW)
    \end{abbrv}

\subsection{Constraints}

    \paragraph{Generation resource constraints}
        
        \begin{enumerate}
            \item Energy step clearing
            \begin{align}
                \label{eq:BPM:gen:energy_step_clearing}
                \pg^{k}_{g, t, s} & \leq \CF_{g, t} \pgstep^{k}_{g, t, s} && \forall g, t, s, k
            \end{align}
            \item Energy dispatch target
                \begin{align}
                    \label{eq:BPM:gen:energy_dispatch_target}
                    \pg_{g, t, s} &= \sum_k{\pg^{k}_{g, t, s}} + \CF_{g, t} \pgmin_{g, t, s} && \forall g, t, s
                \end{align}
            \item Cleared regulating reserve
                \begin{align}
                    \label{eq:BPM:gen:cleared_regulating_reserve}
                    2 \reg_{g, t, s} \leq \RF_{g,t} \regAvail_{g,t}(\pgmax_{g, t, s}-\pgmin_{g, t, s})  && \forall g, t, s
                \end{align}
            \item Cleared contingency reserve
                \begin{align}
                    \label{eq:BPM:gen:cleared_contingency_reserve:spin}
                    \spin_{g, t, s}     &\leq \CF_{g,t} \spinAvail_{g,t}(\pgmax_{g, t, s}-\pgmin_{g, t, s})  && \forall g, t, s\\
                    \label{eq:BPM:gen:cleared_contingency_reserve:suppOn}
                    \suppOn_{g, t, s}   &\leq \CF_{g,t} \suppOnAvail_{g,t}(\pgmax_{g, t, s}-\pgmin_{g, t, s})  && \forall g, t, s\\
                    \label{eq:BPM:gen:cleared_contingency_reserve:suppOff}
                    \suppOff_{g, t, s}  &\leq (1-\CF_{g,t}) \suppOffAvail_{g,t} \suppOffmax_{g, t} && \forall g, t, s
                \end{align}
            \item Maximum and minimum limit
                \begin{align}
                    \label{eq:BPM:gen:min_limits}
                    \pg_{g, t, s} - \reg_{g, t, s} - \rcdn_{g, t, s} &\geq \CF_{g,t} \pgmin_{g,t,s} && \forall g, t, s\\
                    \label{eq:BPM:gen:max_limits}
                    \pg_{g, t, s} + \reg_{g, t, s} + \spin_{g,t,s} + \suppOn_{g,t,s} + \rcup_{g, t, s} &\leq \CF_{g,t} \pgmax_{g,t,s} && \forall g, t, s
                \end{align}
            \item Ramp-up and -down
                \begin{align}
                    \label{eq:BPM:gen:ramp_up}
                    \pg_{g,t+1,s} &\leq \pg_{g,t,s} + \dt \, \rrup_{g,t} && \forall g, t, s \\
                    \label{eq:BPM:gen:ramp_dn}
                    \pg_{g,t+1,s} &\geq \pg_{g,t,s} - \dt \, \rrdn_{g,t} && \forall g, t, s
                \end{align}
            \item Regulating reserve ramp: regulating reserves must be deployable within 5 minutes
                \begin{align}
                    \label{eq:BPM:gen:regulating_reserve_ramp}
                    \reg_{g,t,s} & \leq 5 \times \rrup_{g,t} && \forall g, t, s
                \end{align}
            \item Contingency reserve ramp: contingency reserves must be deployable within 10 minutes
                \begin{align}
                    \label{eq:BPM:gen:contingency_reserve_ramp}
                    \spin_{g,t,s} + \suppOn_{g,t,s} &\leq 10 \times \rrup_{g,t} && \forall g, t, s
                \end{align}
            \item Ramping-up and -down capability: ramping-up and -down capability must be deployable within 10 minutes
                \begin{align}
                    \label{eq:BPM:gen:ramp_up_cap}
                    \rcup_{g,t,s} &\leq 10 \times (1-\ITF_{g,t}) \dt \, \rrup_{g,t} && \forall g, t, s \\
                    \label{eq:BPM:gen:ramp_dn_cap}
                    \rcdn_{g,t,s} &\leq 10 \times (1-\ITF_{g,t}) \dt \, \rrdn_{g,t} && \forall g, t, s
                \end{align}
             \item Short-term ramping capability: short-term ramping capability must be deployable within 30 minutes
                \begin{align}
                    \label{eq:BPM:gen:ramp_str_cap}
                    \rcstr_{g,t,s} &\leq 30 \times (1-\ITF_{g,t}) \dt \, \rrup_{g,t} && \forall g, t, s
                \end{align}
        \end{enumerate}
        
    \paragraph{Reliability constraints}
        \begin{enumerate}
            \item Nodal injection
            \begin{align}
                \label{eq:BPM:rel:nodal_power_balance}
                \p_{i,t,s} &= \sum_{g \in \mathcal{G}_{i}} \pg_{g,t,s} - \pd_{i,t,s} && \forall i, t, s
            \end{align}
            \item Global power balance
            \begin{align}
                \label{eq:BPM:rel:global_power_balance}
                \sum_{i \in \mathcal{N}} \p_{i,t,s} &= \dpp_{t, s} -  \dpm_{t,s} && \forall t, s
            \end{align}
            \item Regulating reserve requirements
            \begin{align}
                \label{eq:BPM:rel:regres_req}
                \sum_{g \in \mathcal{G}}\reg_{g,t,s} & \geq \regReq_{t} - \dreg_{t,s} && \forall t, s
            \end{align}
            \item Regulating plus spinning reserve requirements
            \begin{align}
                \label{eq:BPM:rel:regspin_req}
                \sum_{g \in \mathcal{G}} \left(
                    \reg_{g,t,s} + \spin_{g,t,s}
                \right)
                & \geq \regSpinReq_{t} - \dregspin_{t,s}
                && \forall t, s
            \end{align}
            \item Operating reserve requirements
            \begin{align}
                \label{eq:BPM:rel:op_res_req}
                \sum_{g \in \mathcal{G}} \left(
                    \reg_{g,t,s} + \spin_{g,t,s} + \suppOn_{g,t,s} + \suppOff_{g,t,s}
                \right)
                & \geq \opResReq_{t} - \dopres_{t, s}
                && \forall t, s
            \end{align}
            \item Ramping-up and -down capability reserve requirements
            \begin{align}
                \label{eq:BPM:rel:rcup_req}
                \sum_{g \in \mathcal{G}} \left(
                    \rcup_{g,t,s}
                \right)
                & \geq \rcupReq_{t} - \drcup_{t, s}
                && \forall t, s \\
                \label{eq:BPM:rel:rcdn_req}
                \sum_{g \in \mathcal{G}} \left(
                    \rcdn_{g,t,s}
                \right)
                & \geq \rcdnReq_{t} - \drcdn_{t, s}
                && \forall t, s
            \end{align}
            \item Short-term ramping capability reserve requirements
            \begin{align}
                \label{eq:BPM:rel:rcstr_req}
                \sum_{g \in \mathcal{G}} \left(
                    \rcstr_{g,t,s}
                \right)
                & \geq \rcstrReq_{t} - \drcstr_{t, s}
                && \forall t, s
            \end{align}
        \end{enumerate}
            
    \paragraph{Transmission constraints}
    \begin{enumerate}
        \item PTDF 
        \begin{align}
            \label{eq:BPM:transmission:PTDF}
            \pf_{e, t, s} &= \sum_{i \in \mathcal{N}} \sigma_{e,i} \p_{i, t, s} && \forall e, t, s
        \end{align}
        \item Flowgate limits
        \begin{align}
            \label{eq:BPM:transmission:flow_limits}
            \pfmin_{e,t} - \df_{e, t, s} &\leq \pf_{e,t,s} \leq \pfmax_{e,t} + \df_{e, t, s} && \forall e, t, s
        \end{align}
    \end{enumerate}

    \paragraph{Non-anticipatory constraints}
        \begin{align}
            \pg_{g, 1, s_1}       &= \pg_{g,1,s_2}      && \forall g \in \mathcal{G}, s_1, s_2 \in \mathcal{S} \\
            \reg_{g, 1, s_1}      &= \reg_{g,1,s_2}     && \forall g \in \mathcal{G}, s_1, s_2 \in \mathcal{S} \\
            \spin_{g, 1, s_1}     &= \spin_{g,1,s_2}    && \forall g \in \mathcal{G}, s_1, s_2 \in \mathcal{S} \\
            \suppOn_{g, 1, s_1}   &= \suppOn_{g,1,s_2}  && \forall g \in \mathcal{G}, s_1, s_2 \in \mathcal{S} \\
            \suppOff_{g, 1, s_1}  &= \suppOff_{g,1,s_2} && \forall g \in \mathcal{G}, s_1, s_2 \in \mathcal{S} \\
            \rcup_{g, 1, s_1}     &= \rcup_{g,1,s_2}    && \forall g \in \mathcal{G}, s_1, s_2 \in \mathcal{S} \\
            \rcdn_{g, 1, s_1}     &= \rcdn_{g,1,s_2}    && \forall g \in \mathcal{G}, s_1, s_2 \in \mathcal{S} \\
            \rcstr_{g, 1, s_1}    &= \rcstr_{g,1,s_2}   && \forall g \in \mathcal{G}, s_1, s_2 \in \mathcal{S}
        \end{align}

    \paragraph{Non-negative variables constraints}
        \begin{align}
            \pgstep^{k}_{g, t, s}   &\ge 0      && \forall g, t, s, k\\
            \reg_{g, t, s}          &\ge 0      && \forall g, t, s\\
            \spin_{g, t, s}         &\ge 0      && \forall g, t, s\\
            \suppOn_{g, t, s}       &\ge 0      && \forall g, t, s\\
            \suppOff_{g, t, s}      &\ge 0      && \forall g, t, s\\
            \rcup_{g, t, s}         &\ge 0      && \forall g, t, s\\
            \rcdn_{g, t, s}         &\ge 0      && \forall g, t, s\\
            \rcstr_{g, t, s}        &\ge 0      && \forall g, t, s\\
            \dpp_{t,s}              &\ge 0      && \forall t, s\\
            \dpm_{t,s}              &\ge 0      && \forall t, s\\
            \dreg_{t,s}             &\ge 0      && \forall t, s\\
            \dregspin_{t,s}         &\ge 0      && \forall t, s\\
            \dopres_{t,s}           &\ge 0      && \forall t, s\\
            \drcup_{t,s}            &\ge 0      && \forall t, s\\
            \drcdn_{t,s}            &\ge 0      && \forall t, s\\
            \drcstr_{t,s}           &\ge 0      && \forall t, s\\
            \df_{e,t,s}             &\ge 0      && \forall e, t, s
        \end{align}
    
\subsection{Objective}

    The objective is the sum of the following objective terms.

    \begin{enumerate}
        \item No-load costs
        \begin{align}
            \label{eq:BPM:obj:no-load}
            \sum_{t\in \mathcal{T}} \sum_{g\in \mathcal{G}} \dt \cdot \CF_{g,t} \cdot \noload_{g,t}
        \end{align}
        \item Energy dispatch costs
        \begin{align}
            \label{eq:BPM:obj:dispatch}
            \sum_{g \in \mathcal{G}}\sum_{t \in \mathcal{T}} \sum_{s \in \mathcal{S}} \sum_{k} p_{s} \dt C^{k}_{g,t} \pg^{k} _{g,t,s}
        \end{align}
        \item Reserve procurement costs
        \begin{align}
            \label{eq:BPM:obj:reserves}
            \sum_{g \in \mathcal{G}} \sum_{t \in \mathcal{T}} \sum_{s \in \mathcal{S}} 
                p_{s} \cdot \dt \cdot \text{c}_{g,t,s}
        \end{align}
        where
        \begin{align*}
            \text{c}_{g,t,s}
            &= 
                \costRegRes_{g,t} \reg_{g,t,s}
                + \costSpinRes_{g,t} \spin_{g,t,s}
                + \costSuppOnRes_{g,t} \suppOn_{g,t,s}
                + \costSuppOffRes_{g,t} \suppOff_{g,t,s}
        \end{align*}
        \item Power balance violation penalties
        \begin{align}
            \label{eq:BPM:obj:pen:power_balance}
            \sum_{t\in \mathcal{T}}\sum_{s \in \mathcal{S}} p_{s} \, \dt \, \left(
                \penaltyPowerShortage \dpm_{t,s}
                + \penaltyPowerSurplus \dpp_{t,s}
            \right)
        \end{align}
        \item Regulating reserve shortage penalties
        \begin{align}
            \label{eq:BPM:obj:pen:reg_reserves}
            \sum_{t \in \mathcal{T}} \sum_{s \in \mathcal{S}} p_{s} \, \dt \, \penaltyRegRes\dreg_{t,s}
        \end{align}
        \item Regulating-plus-spinning reserve shortage penalties
        \begin{align}
            \label{eq:BPM:obj:pen:regspin_reserves}
            \sum_{t \in \mathcal{T}} \sum_{s \in \mathcal{S}} p_{s} \, \dt \, \penaltyRegSpinRes\dregspin_{t,s}
        \end{align}
        \item Operating reserve shortage penalties
        \begin{align}
            \label{eq:BPM:obj:pen:op_reserves}
            \sum_{t \in \mathcal{T}} \sum_{s \in \mathcal{S}} p_{s} \, \dt \, \penaltyOpRes \dopres_{t,s} 
        \end{align}
        \item Ramping-up and -down capability shortage penalties
        \begin{align}
            \label{eq:BPM:obj:pen:rcup}
            \sum_{t \in \mathcal{T}} \sum_{s \in \mathcal{S}} p_{s} \, \dt \, \penaltyRCUp \drcup_{t,s} \\
            \label{eq:BPM:obj:pen:rcdn}
            \sum_{t \in \mathcal{T}} \sum_{s \in \mathcal{S}} p_{s} \, \dt \, \penaltyRCDn \drcdn_{t,s} 
        \end{align}
        \item Short-term ramping capability shortage penalties
        \begin{align}
            \label{eq:BPM:obj:pen:rcstr}
            \sum_{t \in \mathcal{T}} \sum_{s \in \mathcal{S}} p_{s} \, \dt \, \penaltyRCStr \drcstr_{t,s}
        \end{align}
        \item Thermal limit violation penalties
        \begin{align}
            \label{eq:BPM:obj:pen:flow}
            \sum_{e \in \mathcal{E}} \sum_{t\in \mathcal{T}} \sum_{s \in \mathcal{S}}
                p_{s} \, \dt \, \penaltyFlow_{e,t} \, \df_{e, t, s}
        \end{align}
    \end{enumerate}
